# Supplementary material for: InsertionNet -- A Scalable Solution for Insertion
Source: arXiv:2104.14223 source file (2021-04-29)
Supplement: Supplementary file 1 [file appendix.tex]

\appendix[Statistical results and analysis]  

%\newpage
SUPPLEMENTARY MATERIAL
\subsection{Simulations: Inserting cylindrical pegs}
\label{M1}
\subsection{Simulations: Inserting cuboid pegs}
\label{M2}
\subsection{Simulations: Inserting smaller  pegs}
\label{M3}
\subsection{Simulations: Inserting pegs with triangle cross-sections}
\label{M4}
\subsection{Real Robot: Inserting different pegs}
\label{M5}
